# Supplementary material for: KL-Entropy-Regularized RL with a Generative Model is Minimax Optimal
Source: arXiv:2205.14211 source file (2022-05-27)
Supplement: Supplementary file 5 [file notations.tex]

\section{Notations}
\label{app:notations}

\begin{table}[h]
	\centering
	\caption{Table of Notations}
	\begin{tabular}{@{}l|l@{}}
		\toprule
		\thead{Notation} & \thead{Meaning} \\ \midrule
	$\A$ & action space of size $A$\\
	$H$ & effective horizon $H \df 1 / (1 - \gamma)$\\
	$P$ & transition matrix\\
	$\X$ & state space of size $X$\\
	$r$ & reward vector bounded by $1$\\
	$\gamma$ & discount factor in $[0, 1)$\\
	\midrule
	$\varepsilon$ & admissible suboptimality\\
	$\delta$ & admissible failure probability\\
	\midrule
	$E_k$ & $E_k : (x, a) \mapsto \sum_{j=1}^k \alpha^{k-j} \varepsilon_j (x, a)$\\
	$\varepsilon_k$ & $\varepsilon_k: (x, a) \mapsto \gamma \widehat{P}_{k-1} v_{k-1} (x, a) - \gamma P v_{k-1} (x, a)$\\
	\midrule
	$A_{k}, A_\infty, A_{\gamma, k}$ & $\sum_{j=0}^{k-1} \alpha^j$, $\sum_{j=0}^{\infty} \alpha^j$, $\sum_{j=0}^{k-1} \alpha^j \gamma^{k-j}$\\
	$\Eone$ & event of small $E_k$ for all $k$ (not variance-aware)\\
	$\Etwo$ & event of small $\varepsilon_k$ for all $k$ (not variance-aware)\\
	$\Ethree$ & event of small $E_k$ for all $k$ (variance-aware)\\
	$\Efour$ & event of small $\varepsilon_k$ for all $k$ (variance-aware)\\
	$\bF_{k, m}$ & $\sigma$-algebra in the filtration (cf.~\cref{sec:main result})\\
	$K$ & number of value updates \\
	$M$ & number of samples per each value update\\
	$P^\pi$ & $P^\pi \df P \pi$\\
	$P^i_j$, $P_*^i$ & $P^i_j \df P^{\pi_i} P^{\pi_{i-1}} \cdots P^{\pi_{j+1}} P^{\pi_j}$, $P_*^i \df (P^{\pi_*})^i$\\
	$T^{\pi}$, $T^i_j$ & Bellman operator for a policy $\pi$, $T^i_j \df T^{\pi_i} T^{\pi_{i-1}} \cdots T^{\pi_{j+1}} T^{\pi_j}$\\
	$V_k$ & an upper bound for $E_k$'s predictive quadratic variance (cf.~\cref{lemma:refined E_k bound}) \\
	$W_k$ & an upper bound for $\varepsilon_k$'s predictive quadratic variance (cf.~\cref{lemma:refined eps_k bound}) \\
	$s_k$ & $s_k \df q_k + \alpha s_{k-1}$ (cf.~\mdvi) \\
	$v_k$ & $v_k \df w_k - \alpha w_{k-1}$ (cf.~\mdvi) \\
    $w_k$ & $w_k (x) \df \max_{a \in \A} s_k (x, a)$ (cf.~\mdvi) \\
    $\alpha$ & $\alpha \df \tau / (\tau + \kappa)$, weight for $s_k$ updates (cf.~\mdvi and \cref{sec:equivalence proof})\\
	$\beta$ & $\beta \df 1 / (\tau + \kappa)$, inverse temperature for $\pi_k$ (cf.~\cref{sec:mdvi} and \cref{sec:equivalence proof})\\
	$\iota_1$, $\iota_2$ & $\iota_1 \df \log (8 K \aXA / \delta)$, $\iota_2 \df \log (16 K \aXA / \delta)$\\
	$\pi_k'$ & a non-stationary policy that follows $\pi_k, \pi_{k-1}, \ldots$ sequentially (cf.~\cref{sec:main result})\\
	$\square$ & an indefinite constant independent of $H$, $\aX$, $\aA$, $\varepsilon$, and $\delta$ \\
	\bottomrule
	\end{tabular}
\end{table}
